# Supplementary material for: Structure and phase boundaries of compressed liquid hydrogen
Source: arXiv:0910.1798 source file (2009-10-09)
Supplement: Supplementary file 1 [file supplemental.pdf]

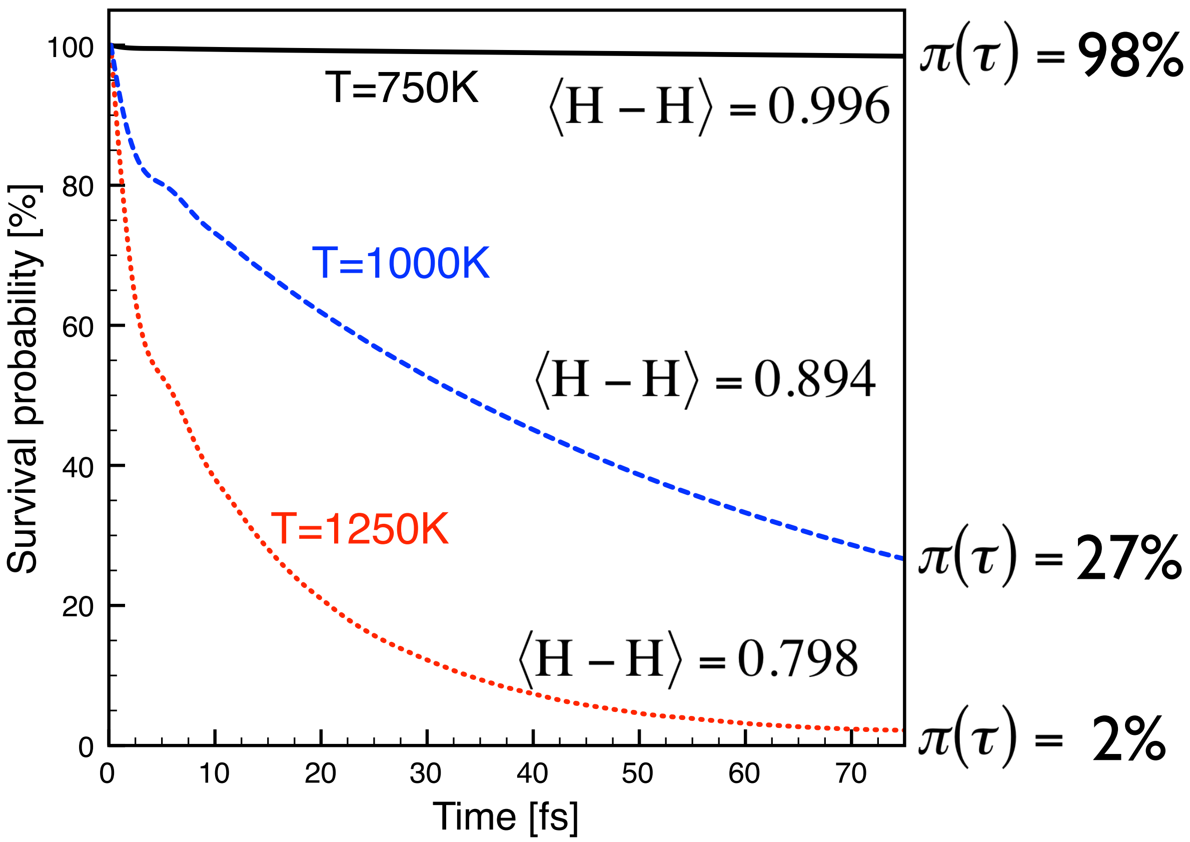


Supplementary Figure 1: Survival probability, $\pi$, as a function of time. Here <H-H> denotes the average fraction of paired (*i.e.* mutual nearest neighbors) H for each temperature. This quantity exhibits a much weaker temperature dependance than $\pi(\tau)$, which is based on the stability of molecules. This plot corresponds to $r_S$=1.40, P ~ 215 GPa.

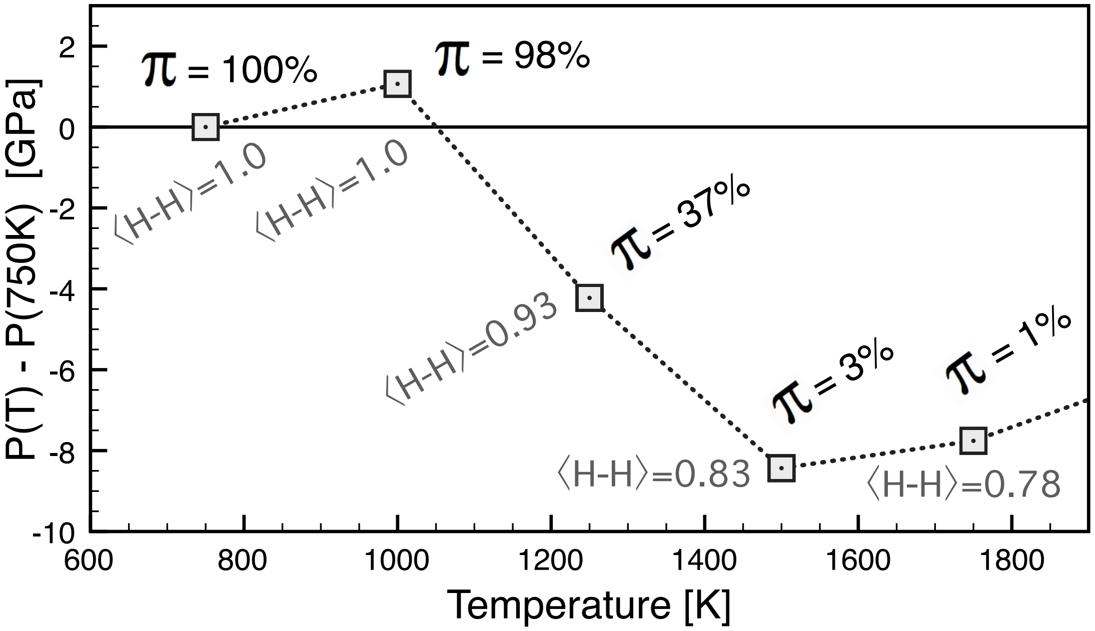


Supplementary Figure 2: EOS of dense liquid hydrogen along an isochore ($r_S$=1.45). Pressures are given relative to the value of $P(r_S=1.45, T=750\text{ K}) = 178.3$ GPa. <H-H> indicates the time average value of mutual nearest neighbors. $\pi$ is the probability for molecules to remain paired after $\tau$ = 76 fs.
